# Supplementary material for: Large Language Model-informed ECG Dual Attention Network for Heart Failure Risk Prediction
Source: arXiv:2403.10581 source file (2024-03-22)
Supplement: Supplementary file 1 [file tmi_appendix.tex]

\documentclass[lettersize,journal]{IEEEtran}
\input{includes.tex}
\input{notations.tex}
 \begin{document}


\appendix
\setcounter{table}{0}
\renewcommand{\thetable}{A\arabic{table}}
\input{appendix}



  \end{document}
